# Supplementary material for: An example of a weakly mixing BV vector field which is not strongly mixing
Source: arXiv:2208.12174 source file (2022-08-25)
Supplement: Supplementary file 1 [file appendix.tex]

\section{Appendix}
\begin{equation}
     \gamma_f=(\rho_c(4)\circ\rho_c(1)\circ e_c(1,2)\circ s^3_c\circ e_c(1,2))\circ(\rho_r(4)\circ\rho_r(1)\circ e_r(1,2)\circ s^3_r\circ e_r(1,2))(\gamma_s).
\end{equation}
\begin{proof}
\begin{equation*}\label{configurations}
   \gamma_s= \left(\begin{matrix}4,1 & 4,2 & 4,3 & 4,4 \\ 3,1 & 3,2 & 3,3 & 3,4 \\ 2,1 & 2,2 & 2,3 & 2,4 \\ 1,1 & 1,2 & 1,3 & 1,4
    \end{matrix}\right)\stackrel{e_r(1,2)}{\longrightarrow}  
    \left(\begin{matrix}4,1 & 4,2 & 4,3 & 4,4 \\ 3,1 & 3,2 & 3,3 & 3,4 \\ 1,4 & 1,3 & 1,2 & 1,1 \\ 2,4 & 2,3 & 2,2 & 2,1
    \end{matrix}\right)\stackrel{s^3_r}{\longrightarrow} 
    \left(\begin{matrix} 2,4 & 2,3 & 2,2 & 2,1 \\  4,1 & 4,2 & 4,3 & 4,4 \\ 3,1 & 3,2 & 3,3 & 3,4 \\ 1,4 & 1,3 & 1,2 & 1,1 \\
    \end{matrix}\right)
\end{equation*}
\begin{equation*}
    \stackrel{e_r(1,2)}{\longrightarrow}  
    \left(\begin{matrix} 2,4 & 2,3 & 2,2 & 2,1 \\  4,1 & 4,2 & 4,3 & 4,4 \\ 1,1 & 1,2 & 1,3 & 1,4 \\ 3,4 & 3,3 & 3,2 & 3,1 \\
    \end{matrix}\right)\stackrel{\rho_r(4)\circ\rho_r(1)}{\longrightarrow}\left(\begin{matrix} 2,1 & 2,2 & 2,3 & 2,4 \\  4,1 & 4,2 & 4,3 & 4,4 \\ 1,1 & 1,2 & 1,3 & 1,4 \\ 3,1 & 3,2 & 3,3 & 3,4 \\
    \end{matrix}\right)\stackrel{e_c(1,2)}{\longrightarrow}
    \left(\begin{matrix} 3,2 & 3,1 & 2,3 & 2,4 \\  1,2 & 1,1 & 4,3 & 4,4 \\ 4,2 & 4,1 & 1,3 & 1,4 \\ 2,2 & 2,1 & 3,3 & 3,4 \\
    \end{matrix}\right)
\end{equation*}
\begin{equation*}
    \stackrel{s^3_c}{\longrightarrow}  \left(\begin{matrix} 3,1 & 2,3 & 2,4 & 3,2\\ 1,1 & 4,3 & 4,4 & 1,2\\ 4,1 & 1,3 & 1,4 & 4,2\\ 2,1 & 3,3 & 3,4 & 2,2
    \end{matrix}\right)\stackrel{e_c(1,2)}{\longrightarrow}\left(\begin{matrix} 3,3 & 2,1 & 2,4 & 3,2\\ 1,3 & 1,1 & 4,4 & 1,2\\ 4,3 & 4,1 & 1,4 & 4,2\\ 2,3 & 3,1 & 3,4 & 2,2
    \end{matrix}\right)
    \stackrel{\rho_c(4)\circ\rho_c(1)}{\longrightarrow}\left(\begin{matrix} 2,3 & 2,1 & 2,4 & 2,2\\ 4,3 & 1,1 & 4,4 & 4,2\\ 1,3 & 4,1 & 1,4 & 1,2\\ 3,3 & 3,1 & 3,4 & 3,2
    \end{matrix}\right)
    \end{equation*}
    c'è da osservare che le colonne sono ordinate come $1,2,3,4$ a metà costruzione. 
\end{proof}
